# Supplementary material for: Computing Nash Equilibria in Potential Games with Private Uncoupled Constraints
Source: arXiv:2402.07797 source file (2024-02-12)
Supplement: Supplementary file 1 [file experiments.tex]

\section{Additional Experiments}

In this section, we present a comprehensive exposition of our experimental methodology, which was briefly introduced in \cref{section:experiments}. We will further elaborate on the setting and visualize two interesting cases, one with maximum constraints applied and one with no constraints. Also, we present the calculation of the Nash gap, provide the results of our hyper-parameter sweep and a demo illustrating the spider charts of all players given private uncoupled constraints.

\subsection{The Setting}
Building upon the initial description provided in \cref{section:experiments}, our experimental setup involves players selecting strategies based on different paths, with the objective of minimizing congestion while considering the gas consumption associated with each option. Specifically, we have five players who make choices among four available routes, each player having their own individual constraint.

In the absence of these constraints, all players would naturally opt for the highway as their best response, given the current configuration. This preference stems from the fact that the congestion penalty for utilizing each edge of the highway is some small constant equal to $0.01$. Even if every player selected the highway, the total congestion would still be less than the congestion experienced by any player deviating to another path, making it the obvious choice for all players, since any other path would yield congestion with a value larger than $2$. However, the introduction of gas constraints serves to diversify the players' actions and compels them to select alternative paths instead of relying solely on the highway.

To calculate the congestion experienced by each player in our congestion game, which involves a total of $E$ edges, we define the potential function:

$$\Phi(\vx) = \sum\limits_{e \in E} \sum\limits_{j=1}^{\ell_e(\vx)} c_e(j)$$

Here, $\ell_e(\mathbf{x})$ denotes the load of each edge $e \in E$, representing the number of players utilizing that particular edge according to the joint policy profile $\mathbf{x}$. The term $c_e(j)$ reflects the congestion experienced on edge $e$ when $j$ players are utilizing it.

\subsection{The Algorithm}
As demonstrated in Algorithm ~\ref{algo}{$\textsc{IGD}{\bm{\lambda}}$\xspace} and formally proven in \cref{lemma:unique_maximizer}, we can effectively solve for the Lagrange multiplier using a closed-form solution. This solution is achievable due to the strong concavity of the Lagrangian with respect to $\vlambda$. Specifically, we have $\vlambda_i^{(t+1)} = \frac{\vg_i(\vx_{i}^{()t})}{2 \mu}$, where $\vg_i(\cdot)$ represents a function and $\mu$ is a parameter. Hence, in contrast to the primal-dual approach, there is no need for an internal loop to approximate $\lambda$.

\subsection{Visualization}

In this section we present two contrasting scenarios to illustrate how the introduction of constraints alters the behaviors of players: one where all players have a surplus of fuel that doesn't infringe any constraints, and another where constraints are imposed maximally. If no constraints existed, minimizing congestion would imply selecting the highway as the congestion on the highway is always less than any other path, even if all players concentrated all of their probability mass on the highway. This is reflected in the plot as all players select the $HW$ path in \cref{fig:constr_off_b} and their corresponding Nash gap in \cref{fig:constr_off_a}.\\
\\
Conversely, the second experiment applies maximum constraints. In this scenario, players are only allowed to select a path with length equal to $2$, effectively allowing $R1$ as the only choice. In \cref{fig:constr_on_b}, we present the spider chart and the corresponding evolution of the Nash Gap over time in \cref{fig:constr_on_a}. Hence, we experimentally verify the convergence to a Nash equilibrium from the Nash Gap plots and the adherence to constraint violations via the spider chart.\\
\\
An intermediate configuration where the gas constraints are distributed between $\min = 2$ and $\max = 10$ is shown in \cref{fig:spider}.
\begin{figure}[t]
    % \centering
    \begin{subfigure}[t]{0.5\textwidth}
        \includegraphics[width=\textwidth]{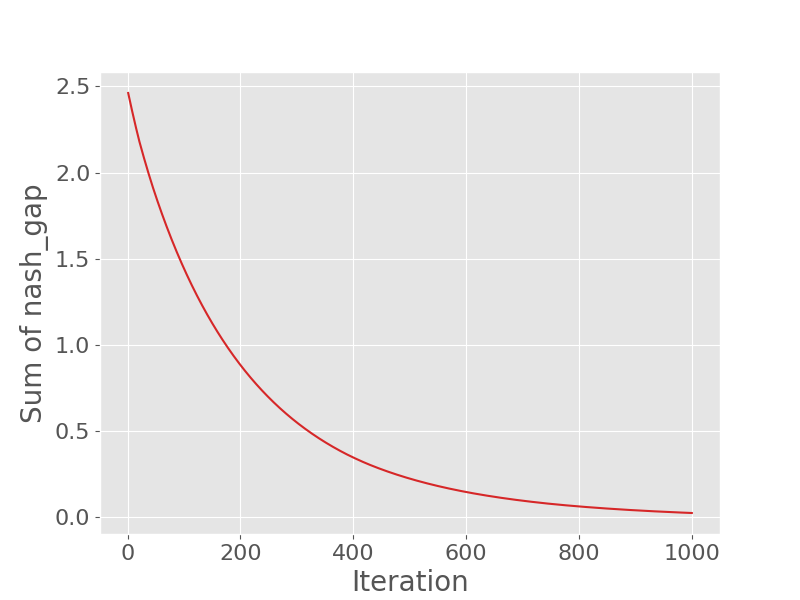}
        \caption{Nash Gap in unconstrained case}
        \label{fig:constr_off_a}
    \end{subfigure}
    \hfill
    \begin{subfigure}[t]{0.5\textwidth}
        \includegraphics[width=\textwidth]{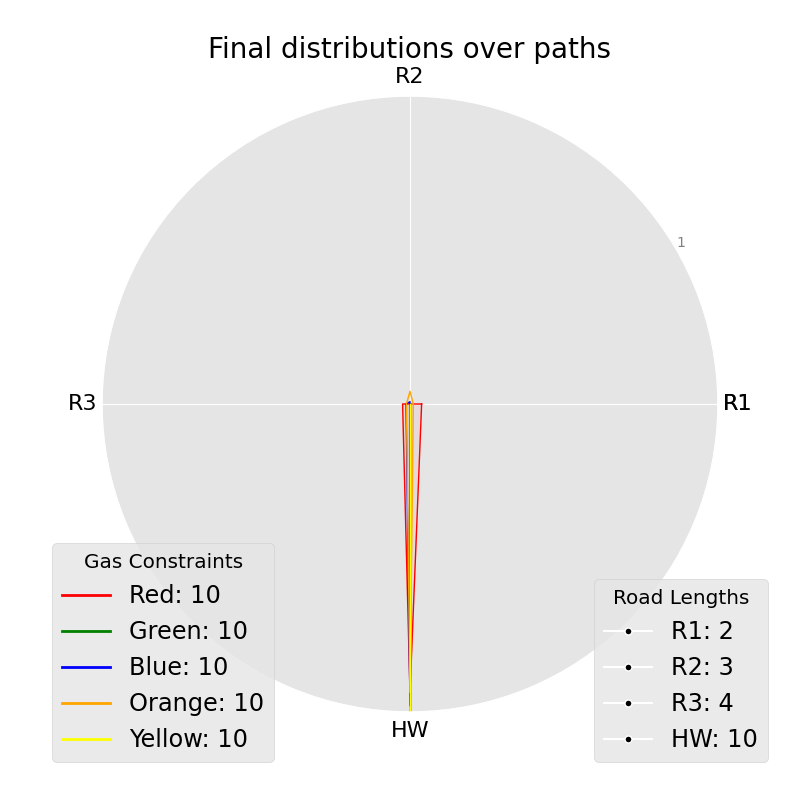}
        \caption{Spider chart of all players in unconstrained case}
        \label{fig:constr_off_b}
    \end{subfigure}
    \caption{Illustration of how players minimize congestion without constraints. All players select the $HW$ path reflecting the highway.}
    \label{fig:constraints_off}
\end{figure}

\begin{figure}[ht]
    % \centering
    \begin{subfigure}[t]{0.4\textwidth}
        \includegraphics[width=\textwidth]{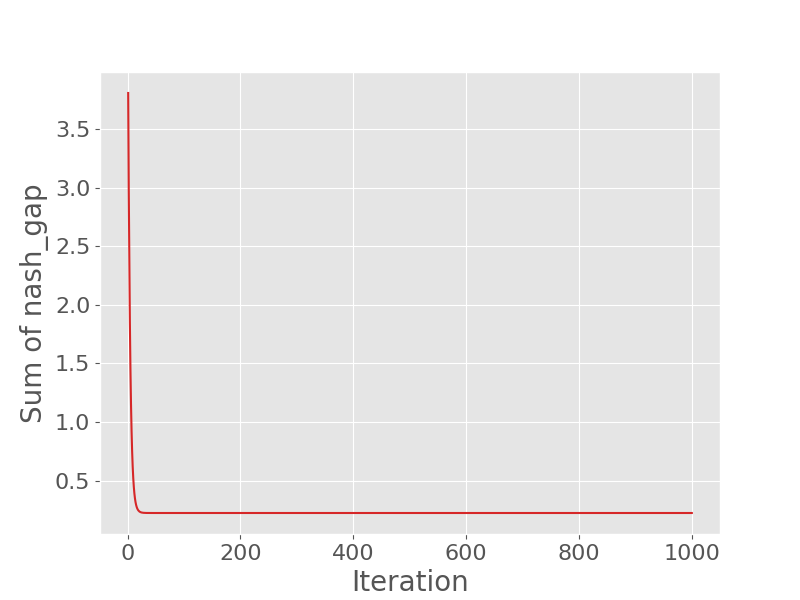}
        \caption{Nash Gap in constrained case}
        \label{fig:constr_on_a} 
    \end{subfigure}
    \hfill
    \begin{subfigure}[t]{0.4\textwidth}
        \includegraphics[width=\textwidth]{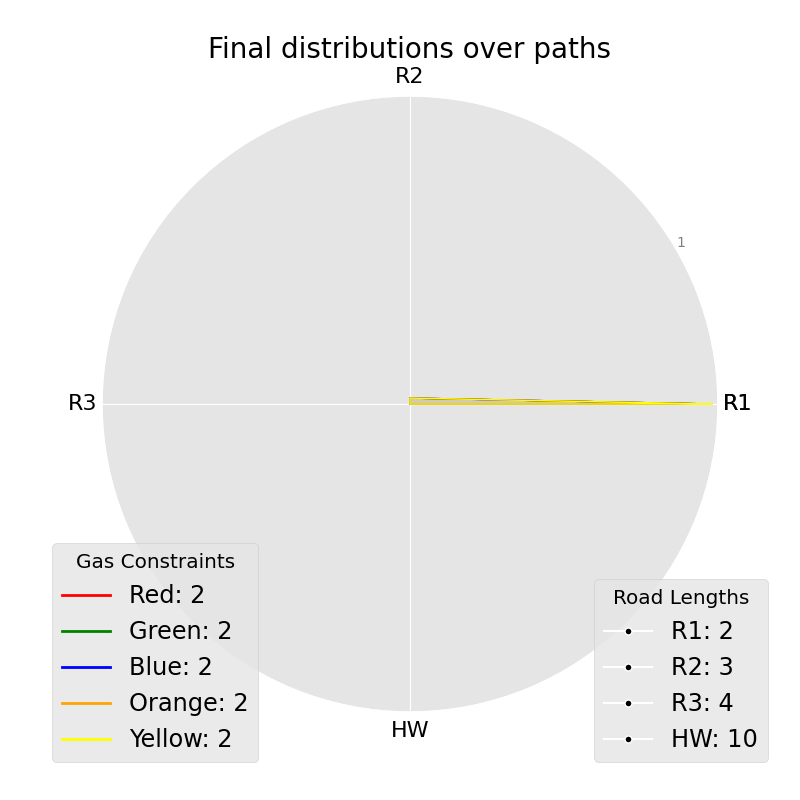}
        \caption{Spider chart of all players in constrained case}
        \label{fig:constr_on_b} 
    \end{subfigure}
    \caption{Illustration of how constraints affect the strategies of all players. In the figure above we select a constraint of $2$ which is the maximum constraint possible for all players. Players do not diversify to minimize congestion and all select $R1$.}
    \label{fig:constraints_on}
\end{figure}
% \newpage
\paragraph{Calculation of Nash gap}
Nash Gap for player $i$ refers to, keeping all players fixed, the difference between the current cost for player $i$ and the cost after player $i$ optimally deviates. Nash Gap in the context of the game is the sum of each player's Nash Gap. 
Nash Gap is defined as follows: 

\begin{equation}
\sum_{i \in \mathcal{N}}
\left(
\min\limits_{\Tilde{\vx}_i \in \Delta(\calA_i)} \{ C_i(\Tilde{\vx}_i; \vx_{-i}) 
\}
-
C_i(\vx_i; \vx_{-i})
\right)
\end{equation}

The Nash Gap metric proves to be a valuable measure, as it attains a value of zero precisely at an exact Nash Equilibrium. Initially, when players' strategies are randomly initialized, we anticipate a significantly positive Nash Gap. As the value gradually diminishes over numerous iterations, we can verify the approaching equilibrium by observing the convergence of Nash Gap towards zero. 
Now, our focus shifts to the efficient calculation of Nash Gap at each iteration. To accomplish this, we note that it is straightforward to calculate a player's cost function for any specific strategy. Initially, we perform this calculation for pure strategies and subsequently acknowledge that the value for mixed strategies can be expressed as a linear combination of these pure strategy-derived costs.
Let $\vp \in \mathbb{R}^{\calA_i}$ represent the vector of costs resulting from each pure strategy, denoted as $p_j = C_i(a_j, \vx_{-i})$ where $a_j$ is the pure strategy $j$. We can express the cost function $C_i(\vx_i, \vx_{-i})$ as the dot product of $\vp$ and $\vx_i$: $C_i(\vx_i, \vx_{-i})  = \vp^{\top} \vx_{i}$.

Therefore, when all other players' strategies are fixed, both the cost and reward can be modeled as linear functions and solved using linear programming. Let $i \in \calN$ be an agent, and $\vc_{\vp} \in \mathbb{R}^{\calA_i}$ denote the vector of budget constraints, the linear program can be formulated as follows:

\begin{align}
\min\limits_{\vx_i \in \Delta(\calA_i)} \vp^{\top} \vx_i \\
s.t. \quad \vc_{\vp}^{\top} \vx_i \leq 0 \\
\mathbf{1}^{\top} \, \vx_i = 1\\
\vx_i \succeq \bm{0} 
\end{align}

\subsection*{Hyper-parameter Sweep}
In order to quantify the affect of the parameters of the game, we experimented with configurations of gas constraints, step-sizes, regularizers, and congestion multipliers, as summarized in the table below.
\newline
\begin{center}
    \begin{tabular}{|c|c|}
\hline
\textbf{Hyperparameter} & \textbf{Values} \\
\hline
Gas & 2, 3, 4, 6, 9, 13 \\
\hline
Strategy Step-size & 0.001, 0.005, 0.01 \\
\hline
Regularizer & 0.00005, 0.0001, 0.001, 0.01 \\
\hline
HW Congestion Multiplier & 0.005, 0.01, 0.05, 0.1 \\
\hline

\end{tabular}
\end{center}

\begin{figure}[!t]
    \centering
    \begin{subfigure}[b]{0.3\textwidth}
        \includegraphics[width=\textwidth]{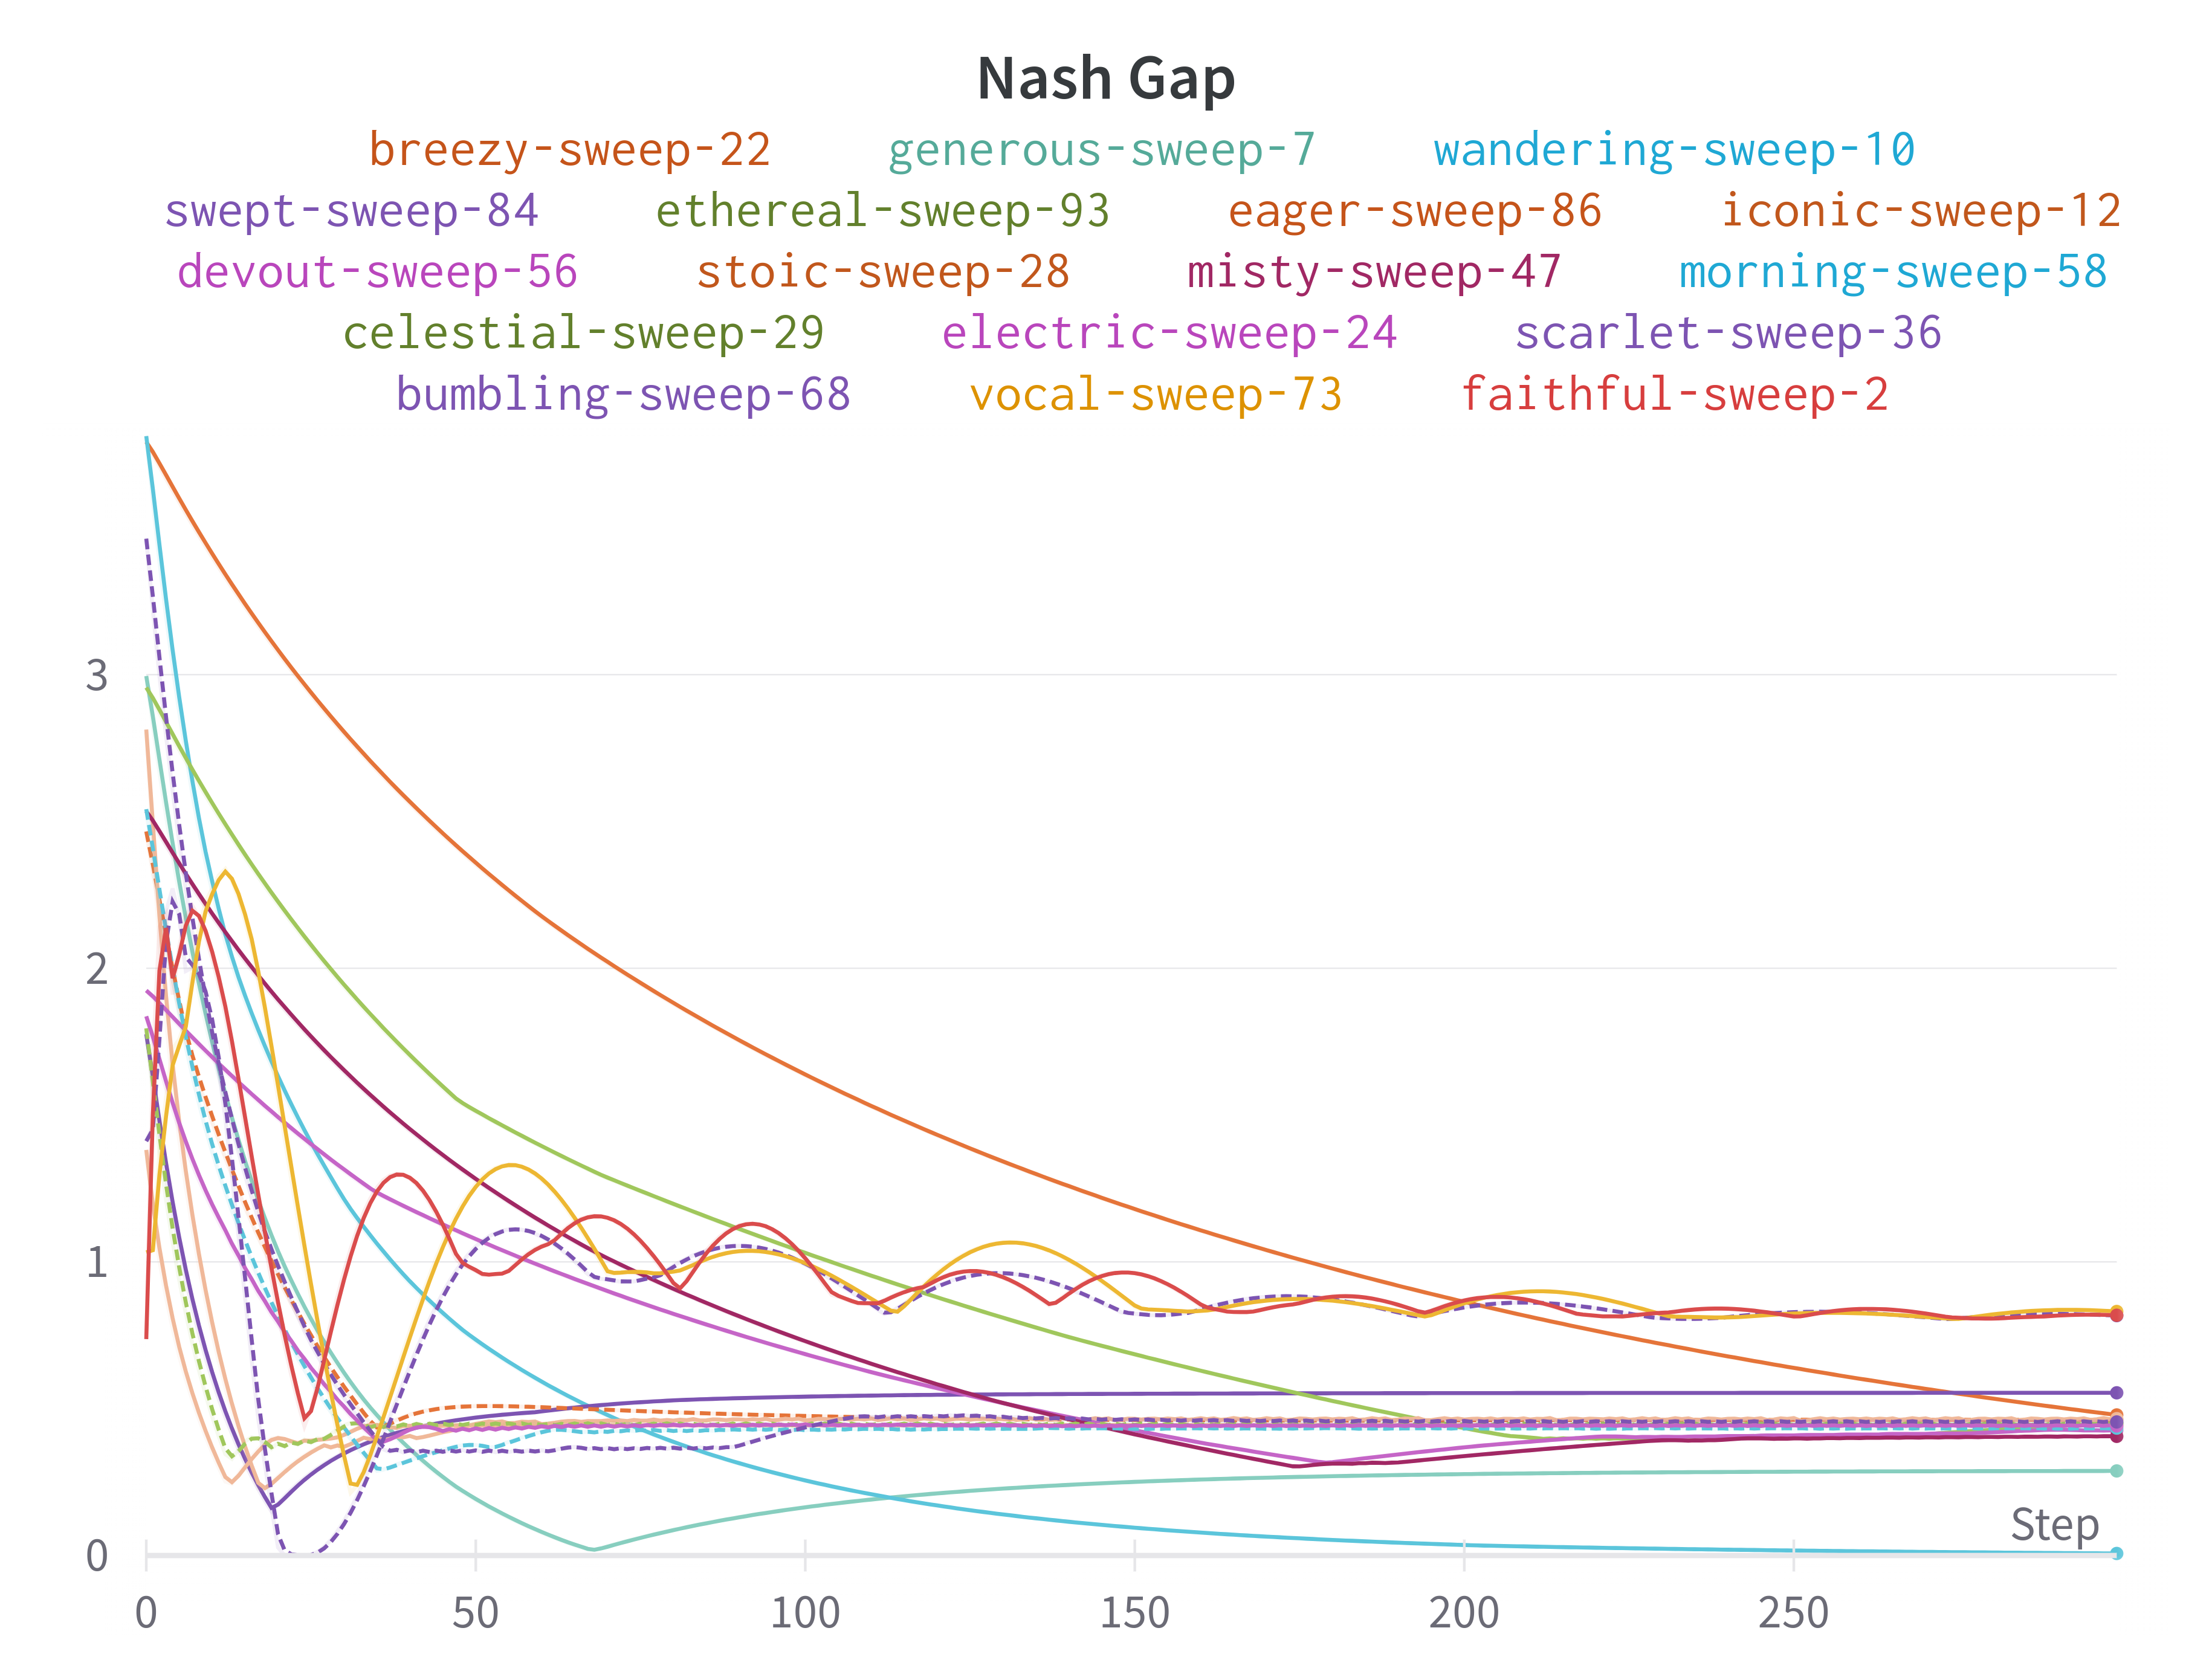}
        \caption{Nash Gap}
        \label{fig:nash_gap_sweep}
    \end{subfigure}
    \hfill
    \begin{subfigure}[b]{0.3\textwidth}
        \includegraphics[width=\textwidth]{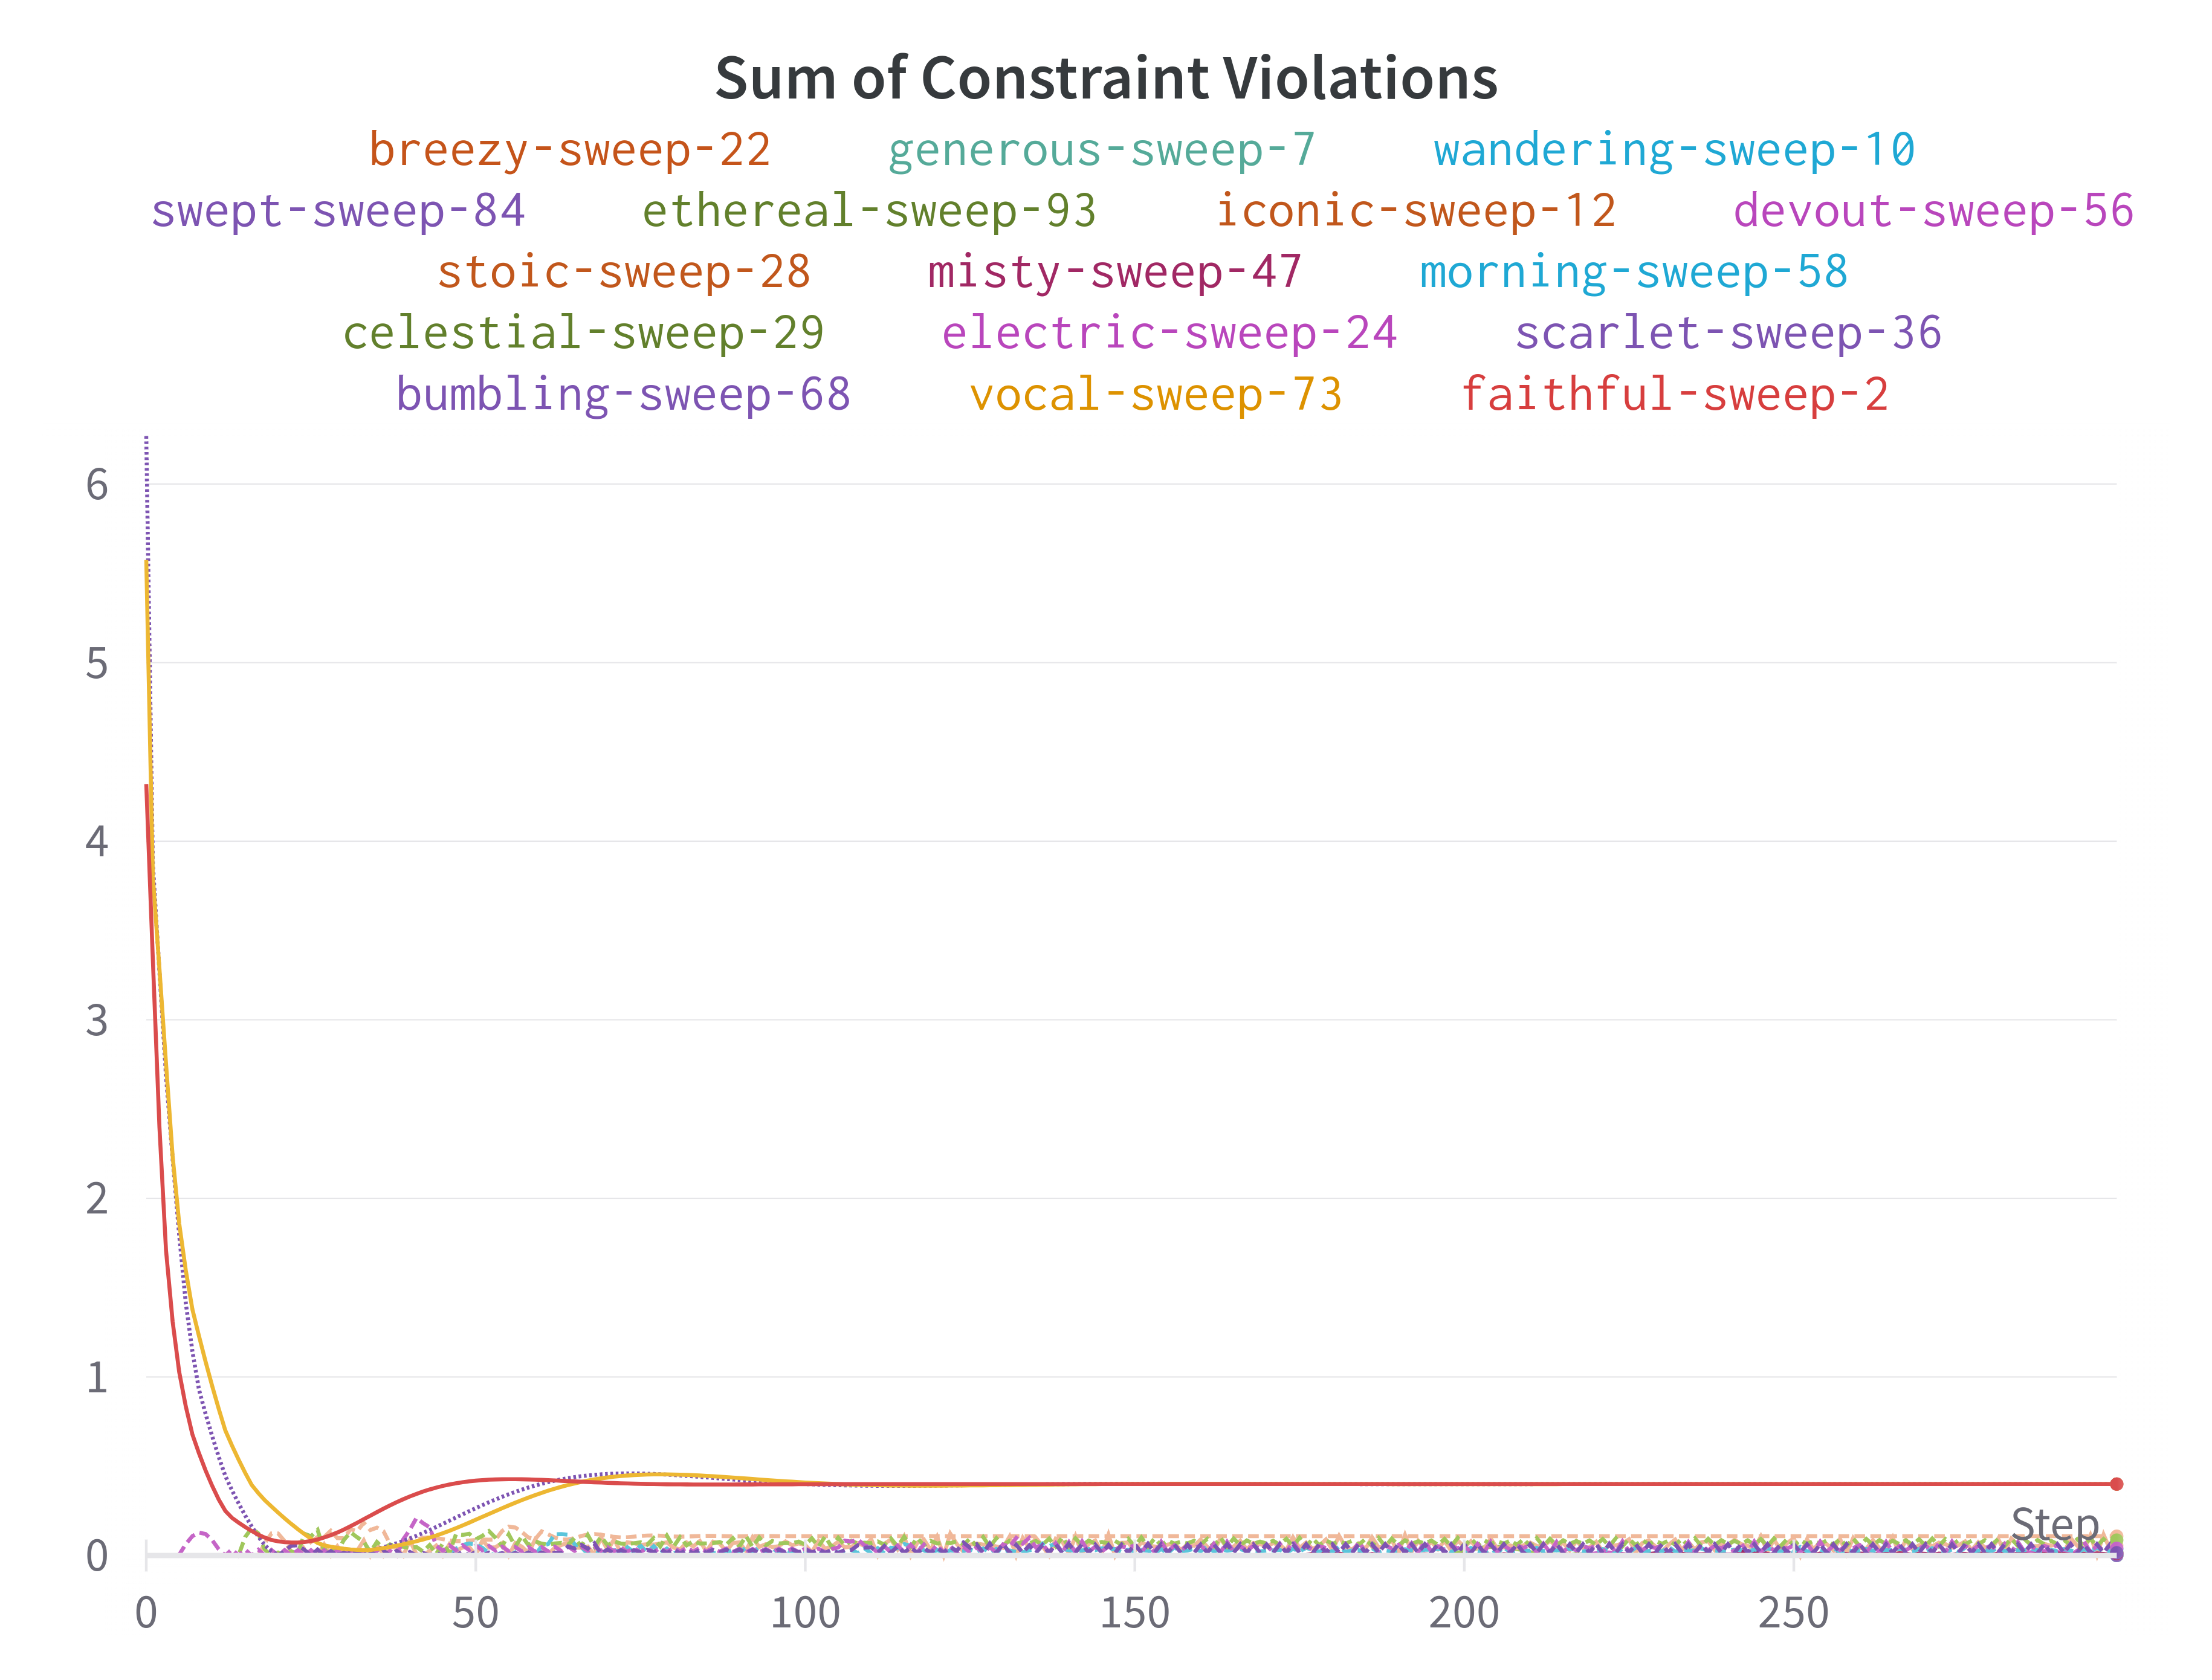}
        \caption{Constraint Violations}
        \label{fig:constraint_violations_sweep}
    \end{subfigure}
    \hfill
    \begin{subfigure}[b]{0.3\textwidth}
        \includegraphics[width=\textwidth]{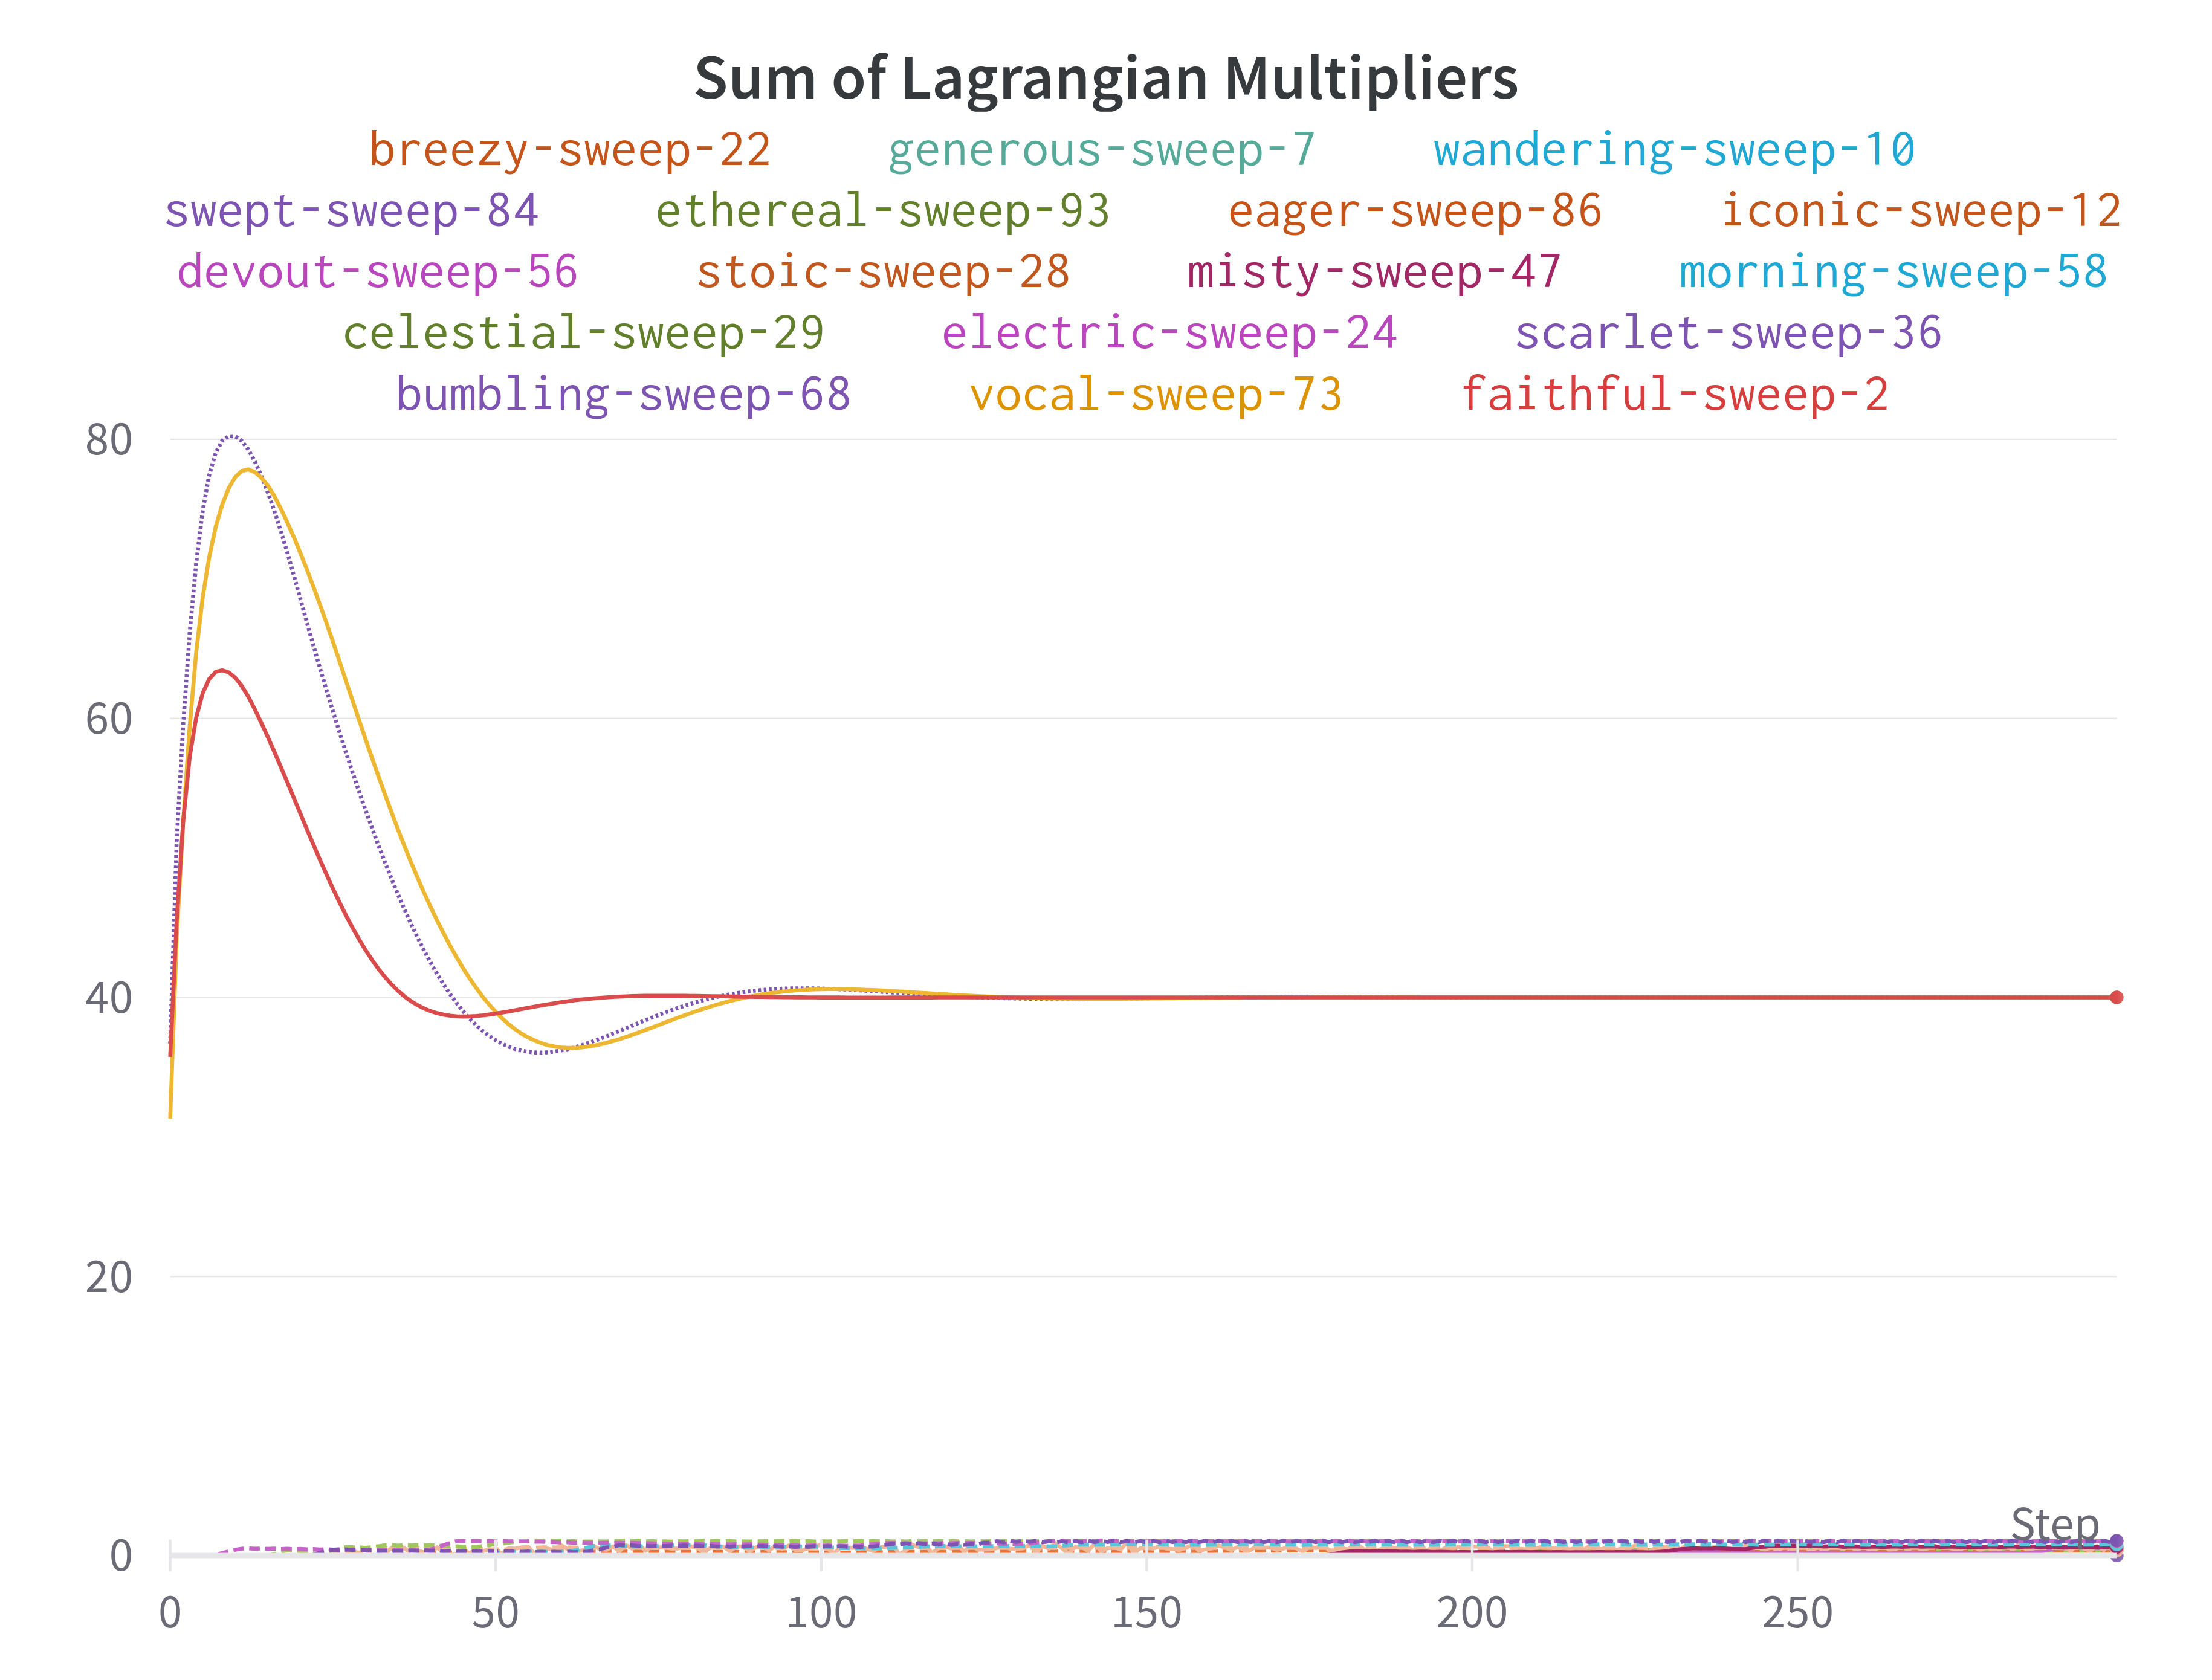}
        \caption{Lagrangian Multipliers}
        \label{fig:lagrangian_multipliers_sweep}
    \end{subfigure}
\end{figure}

We observe that for different configurations of hyper-parameters there is a consistent descending trend of the Nash Gap, the constraint violation approaches zero and the Lagrangian multipliers converge.

% \subsection{Demo}
% The code used for conducting all the experiments can be found in the following online repository:
% https://github.com/steliostavroulakis/constrained-potential-games
% \newline

% The repository houses three interactive jupyter notebooks, including an engaging demo where users can designate constraints and observe the strategies evolving in response, ultimately converging towards an approximate Nash equilibrium. The computing infrastructure used for running experiments are the following:

% \begin{itemize}
%     \item CPU: Intel Xeon CPU at 2.20 GHz
%     \item GPU: - 
%     \item Memory: 13GB
%     \item Operating system: Ubuntu 22.04.3 LTS 
%     \item Python version: 3.10.12
%     % \item Python libraries:
%     % \begin{itemize}
%     %     \item numpy 1.23.5
%     %     \item matplotlib 3.7.1
%     %     \item scipy 1.11.4
%     %     \item networkx 3.2.1
%     % \end{itemize}
% \end{itemize}
