# Supplementary material for: Computing Nash Equilibria in Potential Games with Private Uncoupled Constraints
Source: arXiv:2402.07797 source file (2024-02-12)
Supplement: Supplementary file 2 [file danskin.tex]

\begin{theorem}[Danskin's Theorem \cite{bertsekas1997nonlinear}] 
\label{thm:danskin_theorem}
Let $Z(x)$ be a compact subset of $\mathbb{R}^m$, and let $\phi(x) : \mathbb{R}^n \times Z \rightarrow 
\mathbb{R}$ be continuous and such that $\phi(\cdot, z) : \mathbb{R}^n \rightarrow \mathbb{R}^n$ is convex for each $z \in Z$. Then, the following statements are true.

\begin{enumerate}[label=\roman*.]
\item 
\label{item:danskin_1}
The function $f(x) = \max\limits_{z \in Z} \phi(x,z)$ is convex.

\item 
\label{item:danskin_2}
The directional derivative of $f(x)$ is given by $f'(x;y) = \max\limits_{z \in Z(x)} \phi'(x,z;y)$, where $\phi'(x,z;y)$ is the directional derivative at in $x$ in the direction of $y$, and $Z(x)$ is the set of maximizing points.

\begin{equation} \label{eq:danskin_aux}
Z(x) = 
\Bigl\{ 
\bar{z} \, | \, 
f(x,\bar{z}) = \max\limits_{z \in Z} \phi(x,z) 
\Bigl\}
\end{equation}

\item
\label{item:danskin_3}
If $Z(x)$ in \cref{eq:danskin_aux} consists of a unique point $\bar{z}$ and $\phi(x, \cdot) $ is differentiable at $x$, then $f$ is differentiable at $x$, and it holds,

\begin{equation}
\nabla_x f(x) = \nabla_x \phi(x, \bar{z}).
\end{equation}
\end{enumerate}
\end{theorem}
