# Supplementary material for: Computing Nash Equilibria in Potential Games with Private Uncoupled Constraints
Source: arXiv:2402.07797 source file (2024-02-12)
Supplement: Supplementary file 3 [file experiments_figures.tex]

\begin{figure}[t]
    % \centering
    \begin{subfigure}[t]{0.5\textwidth}
        \includegraphics[width=\textwidth]{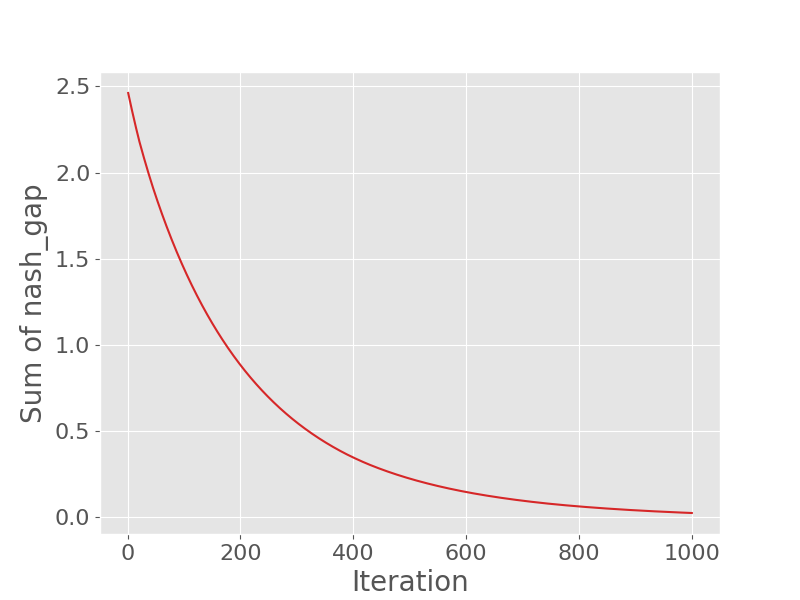}
        \caption{Nash Gap in unconstrained case}
        \label{fig:constr_off_a}
    \end{subfigure}
    \hfill
    \begin{subfigure}[t]{0.5\textwidth}
        \includegraphics[width=\textwidth]{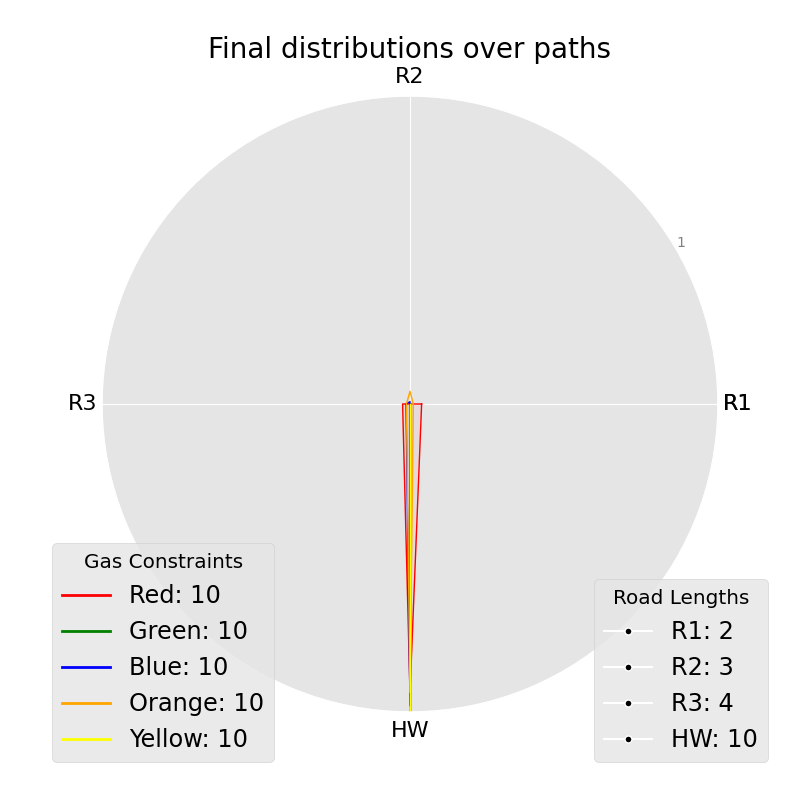}
        \caption{Spider chart of all players in unconstrained case}
        \label{fig:constr_off_b}
    \end{subfigure}
    \caption{Illustration of how players minimize congestion without constraints. All players select the $HW$ path reflecting the highway.}
    \label{fig:constraints_off}
\end{figure}

\begin{figure}[ht]
    % \centering
    \begin{subfigure}[t]{0.4\textwidth}
        \includegraphics[width=\textwidth]{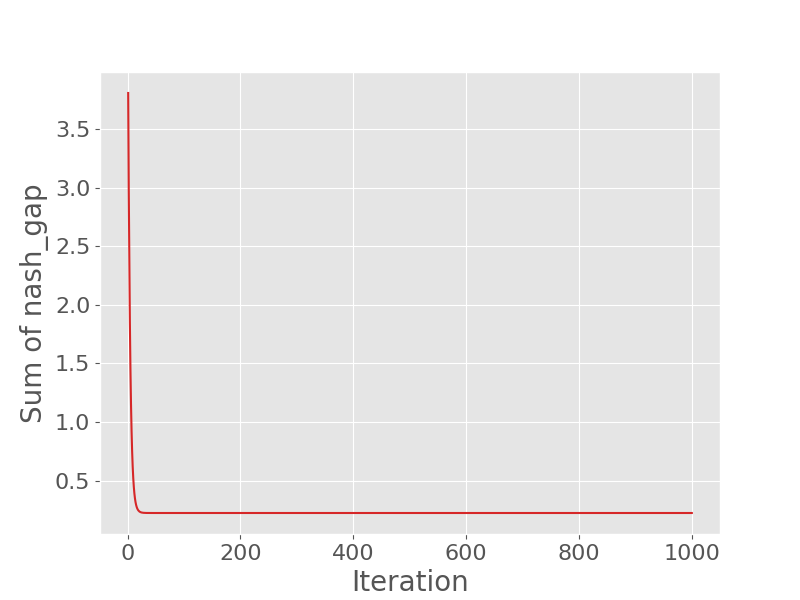}
        \caption{Nash Gap in constrained case}
        \label{fig:constr_on_a} 
    \end{subfigure}
    \hfill
    \begin{subfigure}[t]{0.4\textwidth}
        \includegraphics[width=\textwidth]{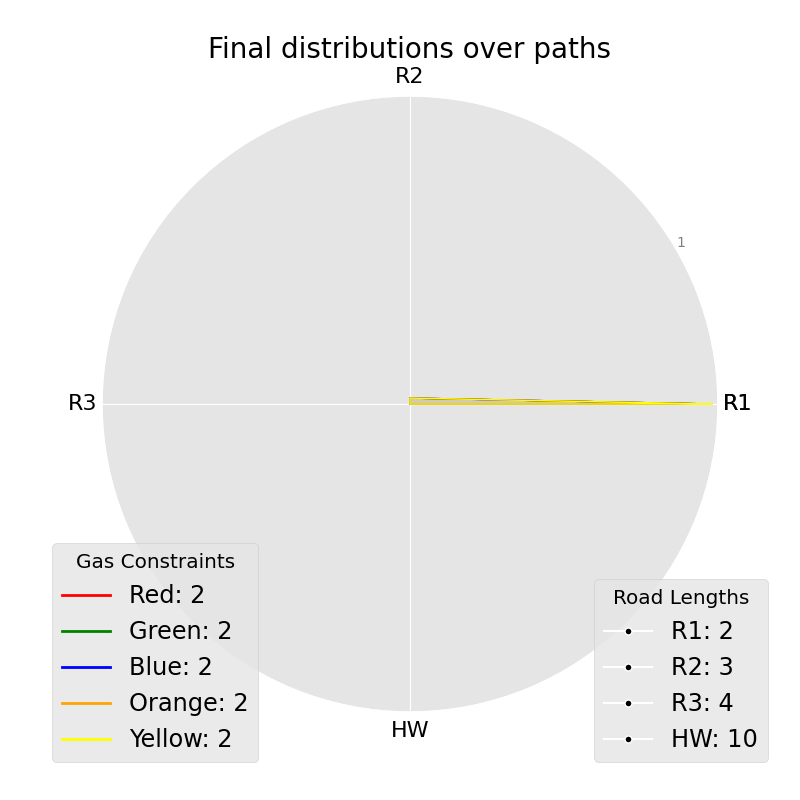}
        \caption{Spider chart of all players in constrained case}
        \label{fig:constr_on_b} 
    \end{subfigure}
    \caption{Illustration of how constraints affect the strategies of all players. In the figure above we select a constraint of $2$ which is the maximum constraint possible for all players. Players do not diversify to minimize congestion and all select $R1$.}
    \label{fig:constraints_on}
\end{figure}
